# Supplementary material for: A Shared Task on Bandit Learning for Machine Translation
Source: arXiv:1707.09050 source file (2017-07-27)
Supplement: Supplementary file 1 [file appendix.tex]

\appendix
\section{Online-to-Batch Conversion}

This shared task focused on the online performance of learning algorithms.  As
mentioned in Section~\ref{sec:eval} (bullet point~\ref{enum:bleu}) the
corpus-BLEU metric is evaluating systems while they are also exploring.  For
the cases when producing a system with a good test performance (e.g.\ for
non-interactive regime) is desirable, this evaluation may not be indicative of
the systems performance in a deployment, exploitation-only, regime.  Hence, one
has to perform online-to-batch conversion to produce a single model to be
deployed.  This can be done by either returning some function of encountered
model, e.g.\ averaged models~\cite{cesa}, random model~\cite{helmbold}, the
longest surviving model~\cite{gallant} or the model that performed the best on
held-out data set~\cite{littlestone}.  Encouraged by the monotonic
development curves (Figure~\ref{fig:dev}) that spoke in favor of the latter
method and taking the final model, we asked the participants to translate a
test set of 7,000 sentences. The results are given in Table~\ref{tab:exploit}. As,
in reality, the training curves were not monotonic (Figure~\ref{fig:train_corpus_bleu}), the final model is
suboptimal for most of the systems, with a possible exception of
SMT-EL-CV-ADAM, that managed to recover the original performance according to
both metrics. 
Note also that 
%for the same reason, as explained in
%Section~\ref{sec:results}, 
there is the same discrepancy between corpus- and
sentence-BLEU results as in Figure~\ref{fig:train_bleu}.

%\todo[inline]{can we have significance tests for non-learning NMT vs best trained SMT systems for the last evaluation on the test set? they seem very close and if they actually get to the same point, that's interesting because their setup is very different}
\begin{table}[!h]
\resizebox{\columnwidth}{!}{
\begin{tabular}{cl|cc|cc}
\toprule
& \multirow{2}{*}{\bf model} & \multicolumn{2}{c|}{\bf corpus-BLEU} & \multicolumn{2}{c}{\bf avg. sent-BLEU} \\
& & \bf before & \bf after & \bf before & \bf after \\
\midrule
& `translate' by copying source & \multicolumn{2}{c|}{0.0425} & \multicolumn{2}{c}{0.0482}\\
\midrule
\midrule
\multirow{5}{*}{\rotatebox{90}{SMT}} & SMT-oracle & \multicolumn{2}{c|}{0.2609} & \multicolumn{2}{c}{0.2800}\\
& SMT-static & \multicolumn{2}{c|}{0.1701} & \multicolumn{2}{c}{0.1601}\\
\cmidrule(r){2-6}
&SMT-EL-CV-ADADELTA& 0.1701 & 0.1635 & 0.1601 & 0.1542\\
%&SMT-EL-CV-ADAM, $\gamma=0.005$    & 0.1701 & 0.1688\\
&SMT-EL-CV-ADAM    & 0.1701 & 0.1707 & 0.1601 & 0.1590\\%$\gamma=0.01$
&SMT-SZO-CV-ADAM   & 0.1701 & 0.1589 & 0.1601 & 0.1512\\%$\gamma=0.005$
%&SMT-SZO-CV-ADAM-T, $\gamma=0.01$  & 0.1701 & 0.1558\\
\midrule
\midrule
%\multirow{8}{*}{\rotatebox{90}{NMT}} & BNMT-oracle, in-data, in-voc & \multicolumn{2}{c|}{0.2893} & \multicolumn{2}{c}{0.3092}\\
\multirow{6}{*}{\rotatebox{90}{NMT}}& BNMT-oracle & \multicolumn{2}{c|}{0.3163} & \multicolumn{2}{c}{0.3297}\\ %cont-in-data, in-voc
%& BNMT-oracle in-data, out-voc & \multicolumn{2}{c|}{0.2794} & \multicolumn{2}{c}{0.2973}\\
& BNMT-static & \multicolumn{2}{c|}{0.1784} & \multicolumn{2}{c}{0.1651} \\
& WMT16-static & \multicolumn{2}{c|}{0.1420} & \multicolumn{2}{c}{0.1246}\\
\cmidrule(r){2-6}
& BNMT-EL-CV & 0.1784 & 0.1226 & 0.1651 & 0.1617\\
& BNMT-EL    & 0.1784 & 0.1491 & 0.1651 & 0.1719\\
& WNMT-EL    & 0.1291 & 0.1321 & 0.1153 & 0.1206\\
%\midrule
%\midrule
%& LIMSI-UCB1          & 0.1729 & 0.0586 & 0.1593 & 0.0350\\
%& LIMSI-UCB1-sampling & 0.1729 & 0.0586 & 0.1593 & 0.0350\\
%& LIMSI-UCB1-select   & 0.1729 & 0.0701 & 0.1593 & 0.0617\\
\bottomrule
\end{tabular}
}
\caption{Results under the exploitation-only mode: Viterbi and greedy inference, respectively, for the SMT and NMT models.}
\label{tab:exploit}
\end{table}
